# Supplementary material for: Situated Understanding of Errors in Older Adults' Interactions with Voice Assistants: A Month-Long, In-Home Study
Source: arXiv:2403.02421 source file (2024-09-23)
Supplement: Supplementary file 1 [file Supplementary_materials.tex]

\section{Findings}
\subsection{Multi-Turn Conversations}
\label{app:findings-multi-turn}
To identify whether participants engaged in multi-turn conversations, we grouped single user query-VA response pairs into multi-turn interactions %\cmh{still do not understand. clear now?? Asked others, it is clear to them}, 
provided the topic remained the same or the participant continued the interaction with the VA; potential multi-turn conversations were identified from recorded audio interactions.

Upon analyzing interactions that were contiguous and centered around the same topic---such as sequences of back-and-forth questions---we identified a substantial number of true multi-turn interactions.
%upon grouping interactions that were contiguous and maintained the same topic---such as multiple back-and-forth questions---we discovered a significant number of multi-turn interactions. 
The continuity in conversations was effectively captured by our recording device, which also aided in discerning if participants had purposefully continued the interaction. Although the majority of interactions (out of 2,552 total turns) were single-turn ($n$ = 1,173), a substantial number involved more than one turn, with 348 instances of two-turn interactions.
Out of the total 2,552 turns, we identified 1,379 instances %(1173 + 348 + \dots) 
%\cmh{this number does not seem to match Fig. 3. NOW IT DOES} 
as being part of multi-turn interactions. Fig. \ref{fig:multi-turn} illustrates the number of turns in these interactions and their frequency. 

\begin{figure*}[t]
     \includegraphics[width=\textwidth]{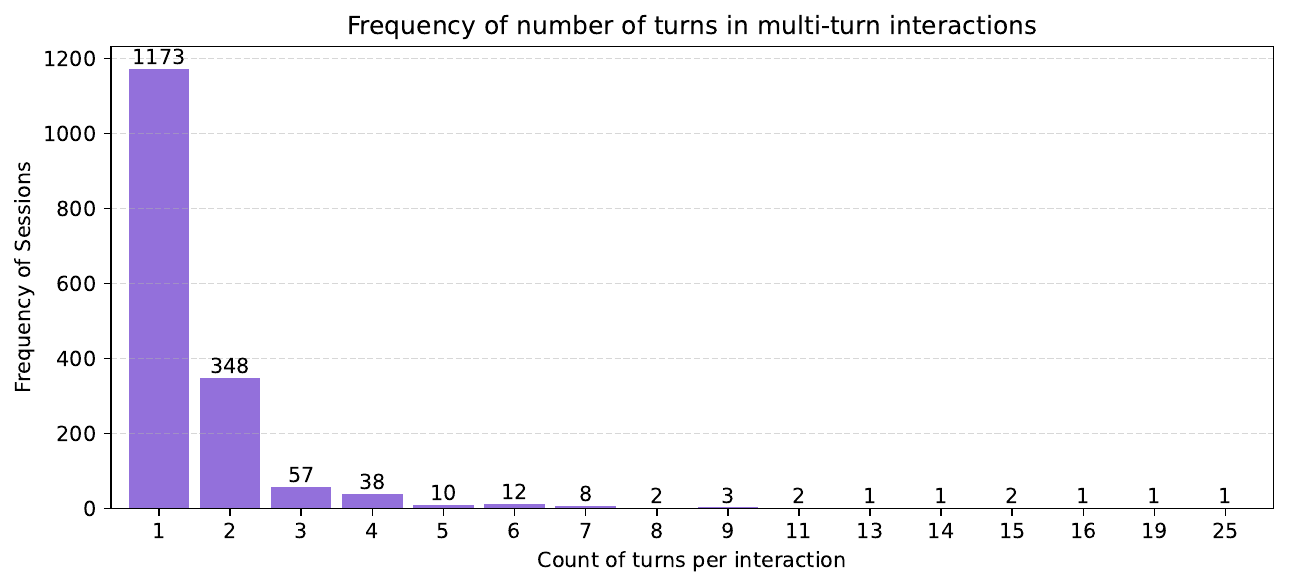}    
     \caption{2,552 total one-turn interactions, 1,379 ($348\times2+57\times3+\dots$) of which were additionally part of multi-turn interactions.}
    
    \label{fig:multi-turn}
\end{figure*}

\subsection{Trends in VA Usage Over Time}
\label{app:findings-usage}
Most of our findings regarding participants' usage patterns confirm prior work \cite{pradhan2020use, kim2021exploring}; below, we provide a comprehensive overview of user engagement with the VA, highlighting any usage trends that emerged over time.
%we present our findings on features of VA that the participants used and how their usage changed over time.  

%\subsection{Older Adults' Usage Patterns: Changes Across Participants}
%\subsubsection{Features in use}

%In our study, we analyzed the types of interactions older adults have with Alexa, a voice assistant, categorizing them based on the nature of the interaction as shown in Table \ref{tab:interaction_categories}. 
%We coded type of interaction for each turn as informed from prior work \cite{pradhan2020use, kim2021exploring}. 
%Interactions were primarily functional ($n=1130$), aiding in memory-related tasks like reminders, timers, calendar updates, and list creation, as well as inquiring about weather and Alexa's capabilities. Entertainment uses ($n=753$), particularly music and radio, were also prevalent. Some participants also engaged Alexa for jokes, stories, and poems. Our findings align with existing literature on older adults' usage of smart speakers \cite{arnold2022does}. 

%The most frequent interaction type was question-asking ($n=414$), primarily for information seeking. These inquiries were further categorized (see Table \ref{tab:question-type}) to understand the nature of information sought \cite{pradhan2020use}, with entertainment-related questions ($n=98$) being the most common. Participants also queried about Alexa itself; for instance, ``how old are you?'' and ``are you a spy?''. 
\subsubsection{Features in use}
\label{sec:findings-features-in-use}
We analyzed the types of interactions older adults had with Alexa and categorized them based on the nature and goal of the interaction as shown in Table \ref{tab:interaction_categories}. 
%We coded type of interaction for each turn as informed from prior work \cite{pradhan2020use, kim2021exploring}. 
Interactions were primarily functional ($n=1130$), aiding with memory-related tasks like reminders, timers, calendar updates, and list creation, as well as inquiries about the weather and Alexa's capabilities; for instance, P15 regularly set reminders for her nightly medication and occasionally queried Alexa to confirm if she had taken her medication or not. Entertainment uses ($n=753$), particularly involving music and radio, were also prevalent. Some participants additionally engaged Alexa for jokes, stories, and poems. 
The most frequent interaction type was question-asking ($n=414$), primarily for the purpose of seeking information; these inquiries were further categorized (see Table \ref{tab:question-type}) to understand the nature of the information sought \cite{pradhan2020use}, with entertainment-related questions (\eg \textit{``Is the Orioles game televised today?''} and \textit{``When was the children's book} Room on the Broom \textit{published?''}) %\cmh{what would be an entertainment question?} 
being the most common ($n=98$). Participants also queried Alexa about itself (\eg \textit{``How old are you?''} and \textit{``Are you a spy?''}).
%Table \ref{tab:alexa-dialogue-questions} \cmh{fix reference }has example conversations of such interactions. 
Our findings align with existing literature on older adults' use of smart speakers \cite{arnold2022does}. \\
%ammari2019music for younger adults
\textbf{Features in use across participants.}
The frequency and nature of interactions varied among participants, as illustrated in Fig. \ref{fig:interaction_categories}. Notably, P5 and couple P10 found limited utility in the device; for example, P5 remarked, \textit{``I couldn't think of ways to use it \dots Maybe I'm not too creative a thinker,''} while P10's usage was affected by one of the pair's full-time employment: ``\textit{Really, I get done with my work day and I really don’t have the time and energy to go exploring new things \dots I’m comfortable interacting with computers, and this was just a new thing that I have to learn that, as I said, I didn't find additional utility in.''}
In contrast, P15 heavily used Alexa for functional tasks, logging 359 interactions---most notably for medication reminders; P15 regularly set reminders for her nightly medication and occasionally queried Alexa to confirm whether she had taken her medication. Entertainment was the second-most frequent use overall, with P3 executing 138 interactions in this category, mostly to listen to music ($n=119$). Participants also exhibited diverse information-seeking behaviors; for instance, P2 had 130 interactions ranging from inquiries about celebrities to probability questions; C1 in Table \ref{tab:alexa-dialogue-errors} provides an example. Additionally, some participants explored more features than others; for instance, P15 wanted to connect her Audible account with Alexa to listen to audiobooks and she also synced her personal calendar to the smart speaker to get audio notifications.

Participants' social interactions with Alexa (\eg expressing gratitude or greeting the device) varied. While some (\eg P6, P15) frequently thanked or greeted Alexa, others (\eg P1, P7, P9, P12) did not engage in such social customs; this variance may reflect differing perceptions of Alexa as a tool versus a social entity. In particular, we observed that P15 used a social response (\eg ``Thank you'') instead of a command (\eg ``Stop'') for her reminders, suggesting a preference for more socially ``polite'' interactions with the device \cite{pradhan2019phantom}.

Couples P12 and P1, who owned multiple smart speakers, showed a more fixed pattern of usage; as documented in Table \ref{tab:tech-use}, they primarily used Alexa for entertainment and functional tasks such as setting timers ($n=22)$ and communication ($n=27)$, with limited experimentation in other functionalities. Interestingly, despite not mentioning this use in their pre-study interviews, they also engaged in information-seeking activities ($n=27$). Similarly, P12 primarily utilized Alexa for entertainment---predominantly for listening to the radio ($n=44$)---and for communication purposes ($n=9$) without exploring additional functionalities.

%TC:ignore
\begin{comment}
    
\begin{table}[tb]
\centering
\caption{Example conversations of question type of interactions ``\dots'' represents truncation of conversation for brevity.  Full conversations are presented in supplementary materials. `CX' is the tag used to refer to the conversations}
\label{tab:alexa-dialogue-questions}
\begin{tabular}{p{0.3cm} M L}
%\hline
\textbf{Tag} & \textbf{Participant} & \textbf{Alexa} \\
\midrule
\midrule

C2 \newline P2& Alexa I've got a math problem what is the likelihood today June the twenty fourth that I will get one hour straight sun?
& In [city], at 11:00 AM, it'll be 76 degrees Fahrenheit with cloudy skies. At 12:00 PM, \dots \\ %it'll be 78 degrees with cloudy skies. At 1:00 PM, it'll be 80 degrees with cloudy skies. At 2:00 PM, it'll be 80 degrees with thunderstorms and mostly cloudy skies.  \\ 
\cdashline{2-3}
 & Alexa you did not answer the math question the answer should come in percentage &  In [city], at 11:00 AM, it'll be 76 degrees Fahrenheit with cloudy skies. At 12:00 PM,  \dots \\ % it'll be 78 degrees with cloudy skies. At 1:00 PM, it'll be 80 degrees with cloudy skies. At 2:00 PM, it'll be 80 degrees with thunderstorms and mostly cloudy skies. \\
\hline

%\multirow{2}{*}{Tag2} & Conversation4 & Pattern4 \\
%\cline{2-3}
%& Conversation5 & Pattern5 \\
%\hline
\end{tabular}
\end{table}
%TC:endignore
\end{comment}

 \begin{figure*}[h]
     \includegraphics[width=\textwidth]{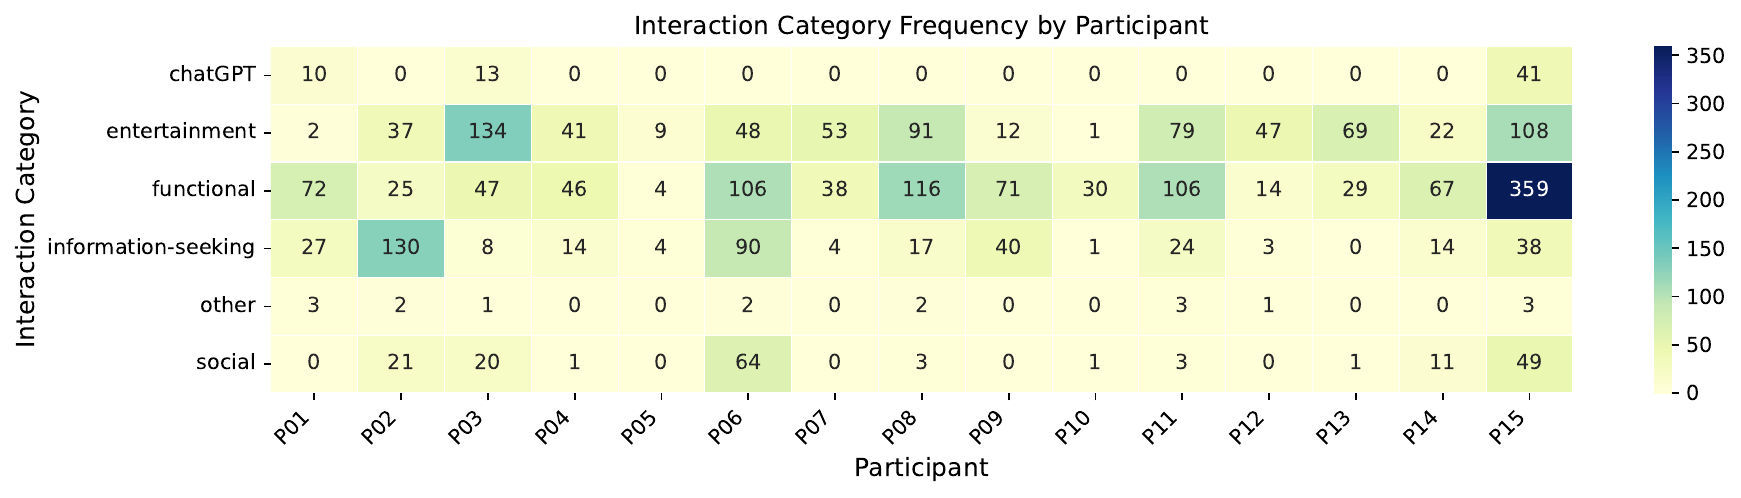}    
     \caption{Types of interactions for each participant.}
    
    \label{fig:interaction_categories}
\end{figure*}

\subsubsection{Usage over time}

\label{app:findings-usage-over-days}

%supports prior work

In examining VA usage trends over time, we considered interaction categories to simplify our analysis (see Fig. \ref{fig:uagaes-over-days}). \\
\textbf{From exploratory behavior to selective use.} %\cmh{unsure how to interpret this heading. From exploratory ... to ...}} 
A notable observation is a decline in overall usage over time, which is consistent with prior work \cite{pradhan2020use, lopatovska2019talk}; participants' initially high usage, characterized by exploratory behavior as the participants experimented with various features, gradually settled into a pattern of utilizing select features that were found to be beneficial in their daily lives. Prior work has discussed factors influencing such a decline in use, including usability issues, forgetting the wake word, and perceived discomfort when talking to a ``machine'' \cite{pradhan2020use}. \\
%evolving user preferences. % [ADD QUOTES ON WHY PEOPLE STOP USING OVER TIME]. 
%%new findings
\textbf{Usage variation across interaction categories.} While looking at the purpose of VA interactions, we found that functional interactions remained the most consistent category over the four-week period, even despite a gradual decline; as functional interactions are need-driven and support daily activities, they tend to integrate more seamlessly into users' routines. In contrast, entertainment-oriented interactions such as listening to music, playing the radio, or asking for jokes exhibited more variability; these desire-driven interactions may be influenced by factors such as mood, available leisure time, and personal preferences, leading to their inconsistent frequency. \\
\textbf{Usage spikes during experimenter check-ins and ChatGPT deployment phase.} Interestingly, we observed spikes in collective usage during specific periods, such as the Week 1 check-in with the experimenter and the ChatGPT deployment phase. These instances suggest that indirect reminders of the VA's presence can temporarily boost usage, although this effect diminishes quickly (as evidenced by the usage peaks in Fig. \ref{fig:uagaes-over-days}).
During the ChatGPT deployment phase, we noticed a spike in usage that can be attributed to participants exploring the new feature; this phase also saw an increase in information retrieval requests using Alexa, possibly for two reasons: 1) failure to activate the ChatGPT skill (\ie forgetting to use the ChatGPT activation phrase ``Let's talk''), resulting in the system defaulting to querying Alexa, %\cmh{still not following the logic here}, 
and/or 2) this phase reminded participants of Alexa's capabilities in answering questions and providing information.

Usage trends over time varied per participant, as well (see Fig. \ref{fig:uagae-over-days-participant}). 
For example, P5 and couple P10 discontinued their use of the device, finding it unhelpful; conversely, some participants---such as P15, P6, and couple P11---engaged with Alexa more consistently, while others like P2 and P3 demonstrated fluctuating patterns of use, with some days seeing more interaction than others.

%The usage trend over days varies for participants as well (see Fig. \ref{fig:uagae-over-days-participant}). P5 and the couple P10 discontinued usage, finding the device unhelpful. Conversely, some participants such as P15, P6, and the couple P11 engaged with Alexa more consistently. While others such as P2 and P3 demonstrated fluctuating patterns of use, with some days seeing more interaction than others.

\subsubsection{Usage at different times of day}

When examining the cumulative four-week data, we analyzed the hours of the day during which users interacted most with Alexa, illustrated in Fig. \ref{fig:uagae-over-hours}. Consistent with previous research \cite{kim2021exploring}, we identified three primary usage peaks: around 8 a.m. (morning), 12 p.m. (noon), and 6 p.m. (evening/night).
%Notably, the evening-night peak exhibited a more spread-out pattern, indicative of varying spare time and night routines among users. This variability is further evidenced by some interactions occurring as late as 1 a.m., reflecting diverse user schedules.
%Furthermore, we observed that functional interactions were more evenly distributed throughout the day compared to entertainment and information-seeking interactions suggesting that functional tasks, being integral to daily routines, are more consistently engaged with at various times. In contrast, entertainment and information-seeking activities showed more concentrated peaks, likely reflecting periods of leisure or specific needs.
Interactions related to the exploration of ChatGPT were predominantly confined to the afternoon, indicating that users tended to experiment with this feature in their spare time, possibly when other commitments were less pressing.

Usage patterns varied across participants, following the findings of prior work \cite{pradhan2020use}; detailed results are presented in Appendix \ref{app:findings-usage}.

 \begin{figure*}[t]
     \includegraphics[width=1.12\textwidth, trim={2.7cm 0 0 0},clip]{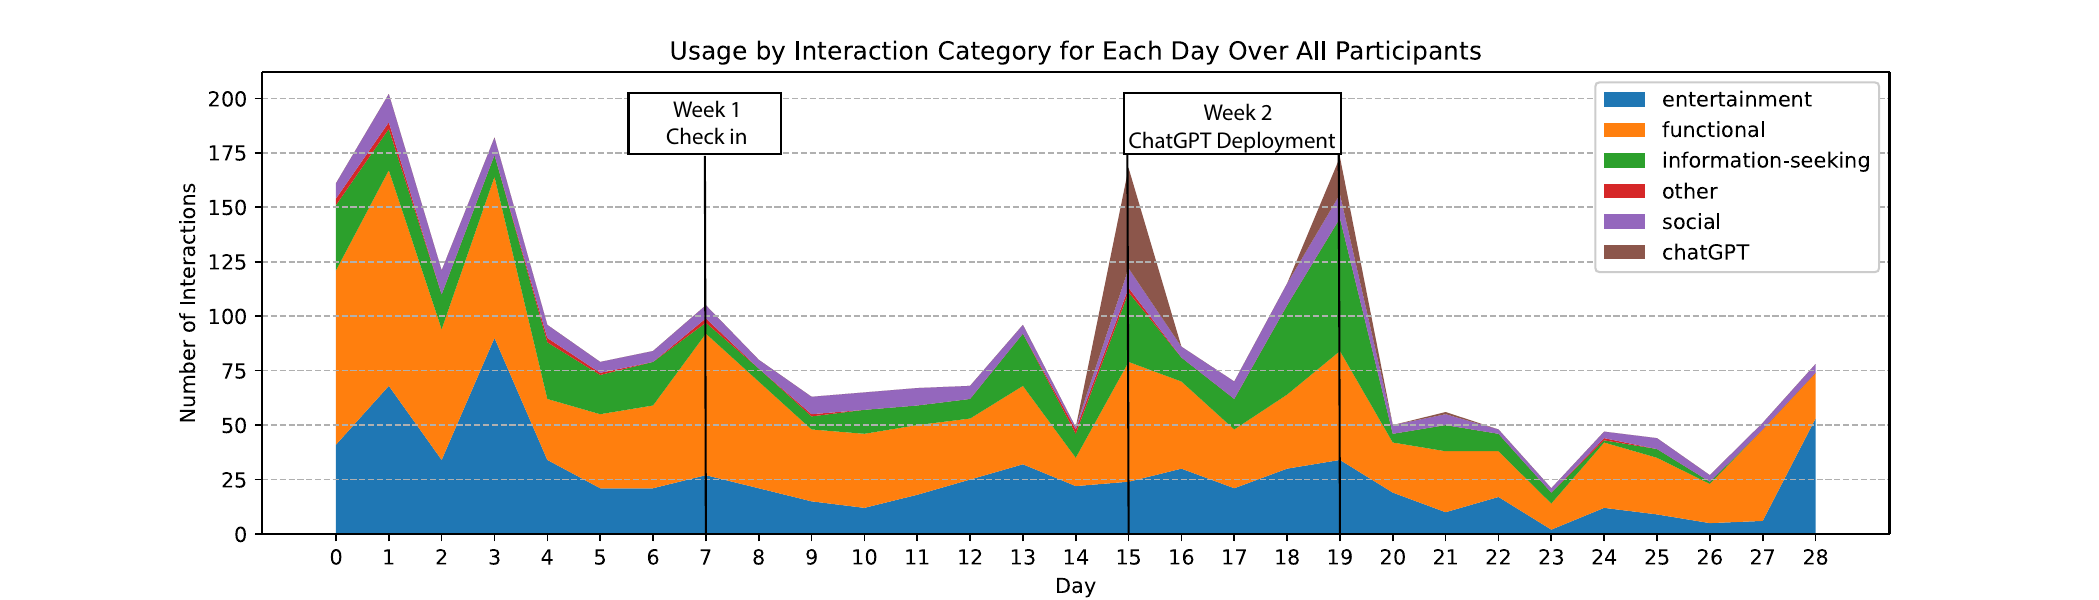}    
     \caption{Interaction categories and their changes in usage over time averaged over all participants.}
    
    \label{fig:uagaes-over-days}
\end{figure*}

 \begin{figure*}[t]
     \includegraphics[width=\textwidth]{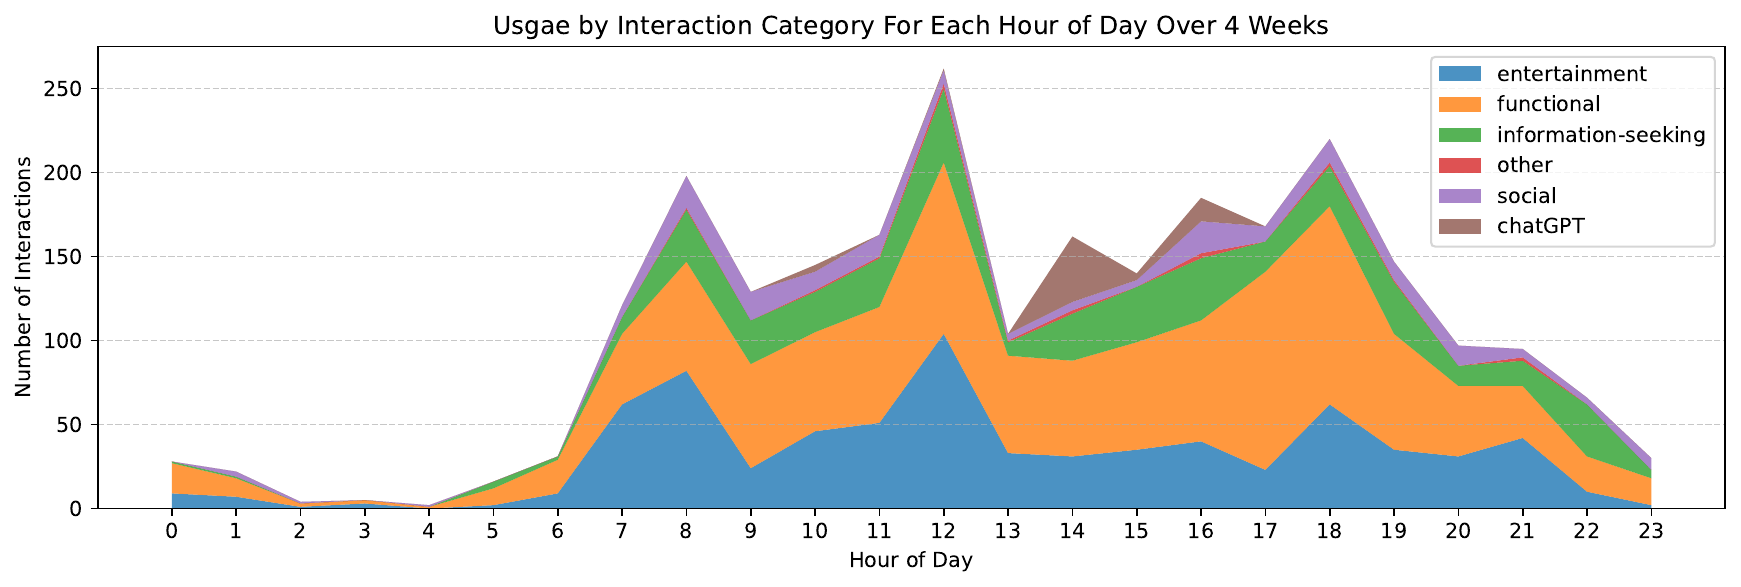}    
     \caption{Interaction categories and their changes in usage over 24 hours averaged over four weeks.}
    
    \label{fig:uagae-over-hours}
\end{figure*}

 \begin{figure*}[t]
     \includegraphics[width=\textwidth]{figures/usage over days participants.pdf}    
     \caption{Changes in participant usage for each day over four weeks.}

    \label{fig:uagae-over-days-participant}
\end{figure*}

%\subsubsection{Usage over times of days}
%\label{app:usage-over-times-of-days}
%In examining the cumulative four-week data, we analyzed the hours of the day during which users interacted with Alexa, as illustrated in Fig. \ref{fig:uagae-over-hours}. Consistent with previous research \cite{kim2021exploring}, we identified three primary usage peaks: around 8 a.m. (morning), 12 p.m. (noon), and 6 p.m. (evening-night). Notably, the evening-night peak exhibited a more spread-out pattern, indicative of varying spare time and night routines among users. This variability is further evidenced by some interactions occurring as late as 1 a.m., reflecting diverse user schedules.

%Furthermore, we observed that functional interactions were more evenly distributed throughout the day compared to entertainment and information-seeking interactions suggesting that functional tasks, being integral to daily routines, are more consistently engaged with at various times. In contrast, entertainment and information-seeking activities showed more concentrated peaks, likely reflecting periods of leisure or specific needs.
%Interactions related to the exploration of ChatGPT were predominantly confined to the afternoon, possibly indicating that users tended to experiment with this feature during their spare time, possibly when other commitments were less pressing.
\subsection{The Social Nature of Voice Interactions }
\label{app:findings-social}
Our audio recordings uncovered new social aspects of VA interactions extending beyond typical use not regularly captured in usage logs; our recordings provide a more situated understanding of users' interactions with the VA and the VA's presence in their daily lives.
%Our audio recordings revealed social aspects of interactions beyond typical VA usage. Such aspects, while can augment the situated understanding of users' interactions with VA, are not usually captured in usage logs otherwise. 

\subsubsection{Social responses and reactions}
\label{sec:social-responses}
Our analysis revealed that participants' interactions with Alexa also included social responses, as detailed in Table \ref{tab:social-responses}. These interactions extended beyond mere task completion. \\
\textbf{Valence of social interactions.} Participants  %often\cmh{compared to the no category, these reactions are not really often.} 
expressed gratitude ($n=179$, \eg ``Thank you''), greeted Alexa ($n=14$, \eg ``Good morning,'' ``Good night,'' etc.), and laughed ($n=13$) at its responses. Additionally, some participants ascribed human characteristics to Alexa because of the way it responded to social interactions, as P14 mentioned: \textit{``When I say, `Thank you, Alexa,' Alexa will say, `Oh, you are welcome, I'm here to serve you.' I don't know why I like to hear that, as if it's a real person or something.''}
We also observed verbal backchannel acknowledgements ($n=20$, \eg ``hmm,'' ``okay'') and participants expressing both positive and negative feedback (backchannel exemplification); positive examples included exclamations of wonder such as \textit{``Isn't that amazing?''} and direct compliments like \textit{``Alexa, I really like you,''} whereas negative feedback was sometimes expressed sarcastically (\eg \textit{``Hell of a job''}) or via critical remarks (\eg \textit{``Alexa is much more stupider''}).
In 21 cases, participants also commented on Alexa's responses or actions (see AC1 and AC2 in Table \ref{tab:alexa-dialogue-private-conversations}).\\
\textbf{Variance across participants.} Participants' social interactions with Alexa varied; while some (\eg P6, P15) frequently thanked or greeted Alexa, others (\eg P1, P7, P9, P12) did not engage in such social customs. This variance may reflect differing perceptions of Alexa as either a tool or a social entity, or it may simply reflect the individual personalities of the participants. \\ %\cmh{or might be just the participant's personality}. \\
\textbf{Social responses as implicit methods of communication.} An interesting observation occurred when P15 used a social response (\ie ``Thank you'') instead of a command (\ie ``Stop'') with her reminders, suggesting a preference for more socially ``polite'' interactions with the VA---a phenomenon also highlighted by prior work \cite{pradhan2019phantom}. Another illustrative example occurred in C12 (Table \ref{tab:alexa-dialogue-errors}), when P15 responded naturally (\eg \textit{``I took my medicine''}) to a ringing reminder to cancel it, but failed to achieve this result. Using a social or natural response instead of a direct command further underscores the tendency of certain individuals to apply implicit communication cues akin to those used in human interactions in their interactions with VAs. Similar behavior was also evident when participants expressed gratitude to the VA even when it failed to fulfill their request, as illustrated in Table \ref{tab:errors-reactions}. The implicit, natural methods of communication used by participants suggest that they may attribute social characteristics to VAs, thus influencing the nature of their communications with them; however, we observed that Alexa often failed to comprehend such implicit communication methods (see C12) even as participants continued to use them, indicating a mismatch between participants' mental models of the VA's capabilities and its actual functionalities.

%\subsubsection{Other social dynamics}
\subsubsection{VAs in social conversations}
\label{sec:social-dynamics}

In our study, we not only observed users' social responses and reactions to Alexa during their interactions with it, but also identified social conversations about Alexa that lent additional insight into the extent of the VA's integration into its users' lives (Table \ref{tab:other-aspects}, left). As examples, we captured participants' discussions about Alexa, instructional conversations on its use, and dialogues stemming from topics initiated with the VA.
Notably, participants typically talked about Alexa ($n=50$) either immediately after or during its use, as depicted in AC3 in Table \ref{tab:alexa-dialogue-private-conversations}.

Additionally, there were 21 instances where participants engaged in discussions on how to operate Alexa with others---more frequently couples trying to navigate its functionality together (C9, Table \ref{tab:alexa-dialogue-private-conversations}) and less frequently when participants were showcasing Alexa to visitors (AC4, Table \ref{tab:alexa-dialogue-private-conversations}).
Participants also engaged in conversations related to topics initiated with Alexa, highlighting the VA's primarily need-based usage and indicating a deeper integration of the system into their daily lives. An illustrative example may be found in couple P11's discussion of the history of Tony Bennett, in which P11a relied on Alexa for information only to find that it did not provide the expected response (C8, Table \ref{tab:alexa-dialogue-private-conversations}); another example occurred in AC5 (Table \ref{tab:alexa-dialogue-private-conversations}), when P1a verified Alexa's answer to P1b's question.

%\subsubsection{Potential negative social interactions}
\subsubsection{Social indicators of friction}
As previously highlighted in Section \ref{sec:error-reactions}, Alexa elicited verbal reactions of a social nature when conversational breakdowns occurred as a result of one or more errors. The elicited social reactions ranged from acknowledgement and laughter to negation and negative commentary to even positive remarks and expressions of gratitude, as detailed in Table \ref{tab:errors-reactions}. Such a diverse array of social responses suggests that participants' interactions with the VA extended beyond mere transactional exchanges.

In addition to reactions to errors, we also captured and coded aspects of participants' interactions that indicated friction in their conversations and that would not typically be captured by usage logs---for instance, interruptions and overlap in both Alexa's and the participants' speech (Table \ref{tab:other-aspects}, right). It is worth noting that most of the interruptions in all the collected interaction data (21 out of 31, as referenced in Tables \ref{tab:errors-reactions} and \ref{tab:other-aspects}) were a direct result of errors made by Alexa.
Despite encountering issues during interactions and the VA's erroneous tendencies as discussed in Section \ref{sec:errors}, our observations revealed minimal overlap and interruptions in participants' speech when interacting with Alexa, suggesting a degree of patience and forgiveness %\cmh{do young adults have this level of patience? something that I have seen is wllingness to work with VA is more in elderly despite more errors than younger adults, that can be reflective of more forgiving behavior} 
toward the VA despite conversational failures. Prior work also reflects a similar sentiment in elderly users---\ie despite experiencing more errors, elderly users tend to exhibit a higher willingness to continue working with voice-based agents in the future as compared to younger adults \cite{barros2020usability}.

%TC:ignore
\begin{table}[t]
    \centering
    \caption{Users' social responses and reactions to Alexa.}
    \label{tab:social-responses}
    \begin{tabular}{lr|lr}
        \toprule
        \textbf{Social Response/Reaction} & \textbf{Count} &\textbf{Social Response/Reaction} &\textbf{Count} \\
        \midrule
        \midrule
        ``No''                                      & 2301 & Greeting                                  & 14 \\
        Gratitude                               & 179  & Laughter                                  & 13 \\
        Remarks                                 & 21   & Verbal backchannel exemplification, negative & 12 \\
        Verbal backchannel acknowledgement      & 20   & Verbal backchannel exemplification, positive & 9  \\
        \bottomrule
    \end{tabular}
\end{table}
%TC:endignore

%TC:ignore
\begin{table}[tb]
\centering
\caption{Conversations exemplifying social aspects beyond simple interactions. ``\dots'' represents the truncation of a conversation for brevity. Full conversations are available in the supplementary materials.}
\label{tab:alexa-dialogue-private-conversations}
\begin{tabular}{p{0.3cm} M L}
%\hline
\textbf{Tag} & \textbf{Participant} & \textbf{Alexa} \\
\midrule
\midrule

AC1 & Alexa, what is Donald Trump's educational background? & Donald Trump was educated at UPenn. \\ %University of Pennsylvania.	\\
\cdashline{2-3}
P2 & \myc{[remarking]} That's it, no Harvard, no Yale. & \myc{[Not heard by Alexa]} \\
 \hline
AC2 & \myc{[User initiates incomplete reminder request.]} & When should I remind you? \\% and is closely related to Chikungunya, O’nyong-nyong, Ross River, Barmah Forest, and Sindbis viruses (1–3). \\
 \cdashline{2-3}
P11b & \myc{[No user response]} & What's the reminder for? \\
 \cdashline{2-3}
 & She remembers it! & \\%, James Biden, and Valerie Biden Owens, and his relative is Valerie Biden Owens. \\
 \hline
AC3 & Alexa, put hard candy on my shopping list.  & You already have hard candy on your shopping list. \\ %University of Pennsylvania.	\\
\cdashline{2-3}
P6 & Oh. \myc{[To visitor:]} Did you hear her? I said, ``Alexa \dots &  \\
 \hline
%C9 & Alexa, give me a 10 minute warning please.  & 10 minutes, starting now \myc{[it worked]} \\ %University of Pennsylvania.	\\
%\cdashline{2-3}
%P11a & & \cellcolor{user} \myc{[P11b to P11a:} No you need to say timer for 10 minutes \myc{[overlapping Alexa speech]}  \\
%\cdashline{2-3}
% & What wait wait what \{P11b's name\} & \cellcolor{user} \myc{[P11b to P11a]:} Set a time for 10 minutes  \\
% \cdashline{2-3}
% & Okay \myc{[To P11b]} Alexa, set timer for 10 minutes & Second timer, 10 minutes, starting now \\
% \cdashline{2-3}
% & Set a time for 10 minutes \myc{[P11b to P11a]} & \\
% \hline
AC4 & Alexa, add milk to my shopping list.  & I added milk to your shopping list. \\ %University of Pennsylvania.	\\
\cdashline{2-3}
P8 & I don't know where the list is. \myc{[Visitor to P8:]} Oh wait a minute, maybe it's in Amazon \dots  &  \\
 \hline
%C8 & Alexa play the history of Tony Bennett.& \cellcolor{user} \myc{[P11b to P11a]:} What's the history of Tony Bennett  \\
%\cdashline{2-3}
% P11a & \myc{[To P11b]} Oh she'll tell you & \cellcolor{user} \myc{[P11b chuckles mockingly]} \\
 \cdashline{2-3}
% & She didn't tell you \myc{[to P11b]}  & \cellcolor{user} \myc{[P11b to P11a]:} Because it makes no sense\\
 \hline
 AC5 \newline P1b & Did the actress who played the voice of Howard Wolowitz on \textit{3rd Rock from the Sun} really die? & From fun107.com: But sadly, the actress behind that memorable voice has passed away. \\
\cdashline{2-3}
 & \myc{[P1a to P1b:]} That is true. She did pass away.  & \\
 \hline
 AC6 \newline P15 & Alexa, tell me a joke. & Sometimes people ask me if I speak lizard. I don't, but iguana learn someday! \\
\cdashline{2-3}
 & \myc{[laughter]} Okay, so you're still working.  & \myc{[Not heard by Alexa]} \\
 \hline

\end{tabular}
\end{table}
%TC:endignore

%TC:ignore
\begin{table}[t]
    \centering
    \caption{Additional aspects of participants' interactions with Alexa.}
    \label{tab:other-aspects}
    \begin{tabular}{lr|lr}
        \toprule
        \textbf{Description }& \textbf{Count} &\textbf{Description} &\textbf{ Count} \\
        \midrule
        \midrule
        Private conversation about Alexa & 50 & Overlap: Participant starts talking over Alexa & 12 \\
        Private conversation about how to use Alexa & 21 & Overlap: Alexa starts talking over participant & 4 \\
        Private conversation about same topic & 15 & Participant interrupts Alexa & 31 \\
        &  & Alexa interrupts participant & 15  \\
        \bottomrule
    \end{tabular}
\end{table}
%TC:endignore
\begin{comment}
    
%TC:ignore
\begin{table}[tb]
\centering
\caption{Additional illustrative conversations.  ``\dots'' represents truncation of conversation for brevity.  }
\label{tab:alexa-dialogue-additional-appendix}
\begin{tabular}{p{0.3cm} S X}
%\hline
\textbf{Tag} & \textbf{Participant} & \textbf{Alexa} \\
\midrule
\midrule

AC6 \newline P15 & Alexa tell me a joke & Sometimes people ask me if I speak lizard. I don't, but iguana learn someday! \\
\cdashline{2-3}
 & \myc{[laughter]} Okay, so you still working  & \myc{[not listened by Alexa]} \\
 \hline

\end{tabular}
\end{table}
%TC:endignore
\end{comment}

%\subsection{Additional Error Analysis}

\begin{figure*}[t]
     \includegraphics[width=\textwidth]{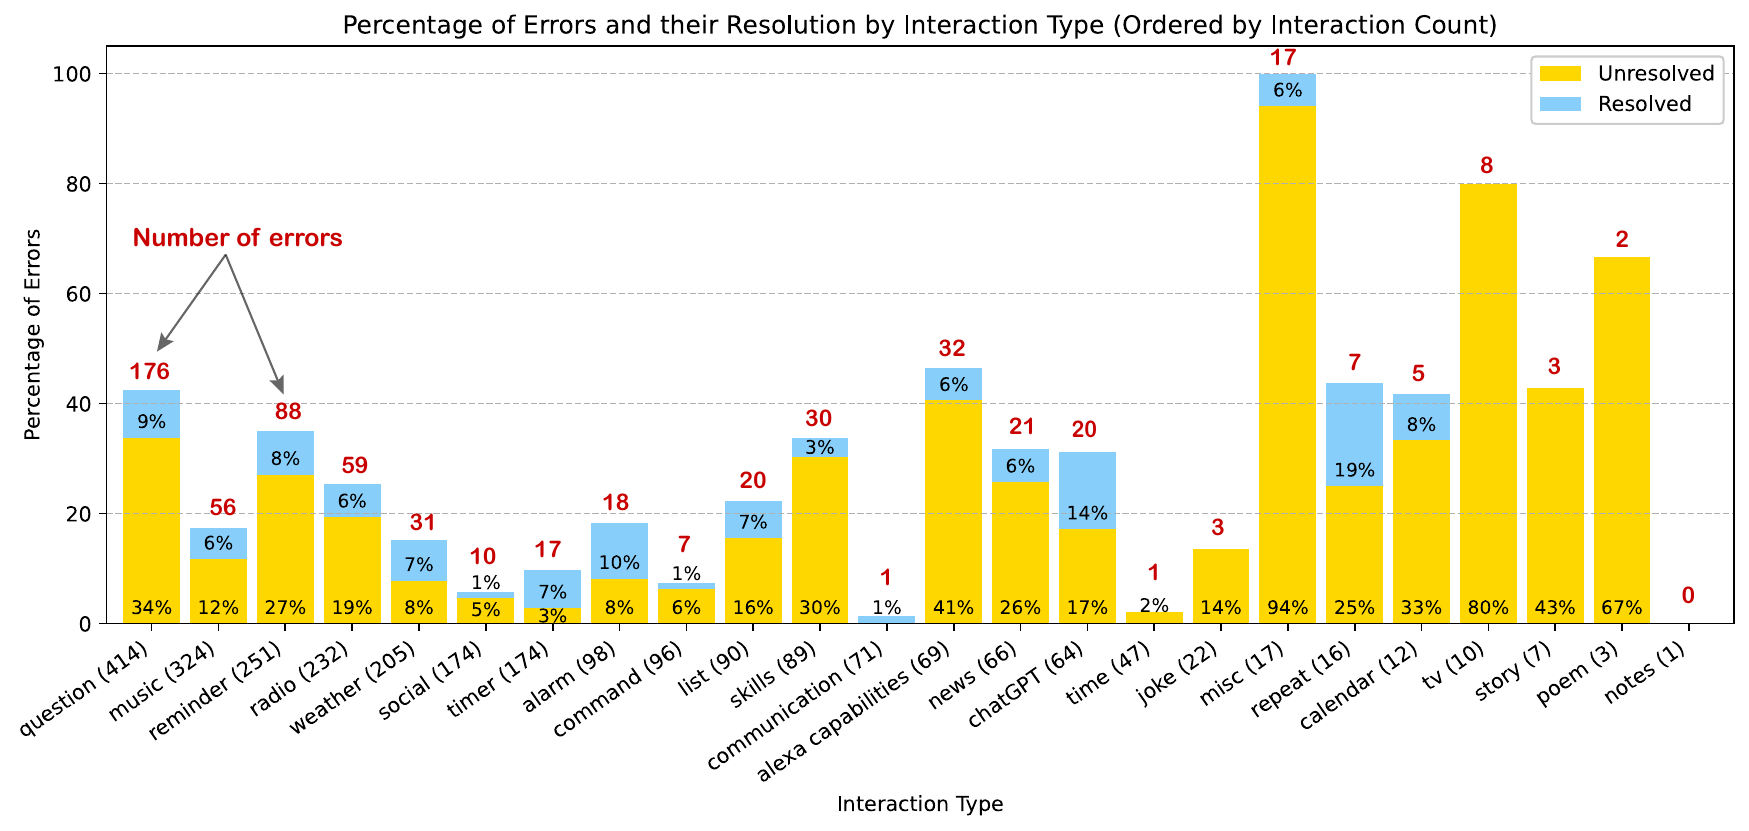}    
     \caption{For each interaction type, the percentage of interactions that resulted in errors and the percentage of interactions in which the error was resolved or not. Interaction types are listed in descending order of their frequency in the interaction data. The number of errors on each bar indicates the total errors in that interaction type. For instance, 414 interactions were of the ``question'' type; 176, or $44\% (34\%+9\%)$ of those resulted in an error; and only $9\% $ of the 414 interactions were resolved after the first retry. Note: Not all errors had retries and some errors had multiple retries, as discussed later.}
    
    \label{fig:errorneous-interactions}
\end{figure*}

\section{Discussion}
\subsection{Voice Assistance in Older Adults' Lives} %as a Social Entity}

Our findings corroborate prior studies demonstrating the utility of VAs in the lives of older adults, particularly for supporting memory through functional tasks, providing entertainment, and delivering necessary information \cite{kim2021exploring, pradhan2020use}. 
Our participants explored a variety of features, reflecting the VA's multifaceted role in their lives; for instance, playing music and listening to news indicate potential uses of voice assistance beyond need-based tasks. Many participants also engaged in creating reminders and shopping lists, pointing to a blend of functional and entertainment uses for the VA. Some participants used Alexa for more diverse purposes, such as attempting to connect it with their Audible account to listen to audiobooks, syncing their personal calendar to stay updated, and asking the system to tell jokes, stories, and poems, suggesting that VAs are perceived not merely as tools but also as ``digital companions''---a perspective that differs from that of younger adults \cite{chung2019elderly}.
Our study also revealed the creative ways in which different participants interacted with the VA. For example, P15 demonstrated an inventive approach by asking Alexa to tell a joke to check whether it was working after a malfunction (AC6, Table \ref{tab:alexa-dialogue-private-conversations}); this particular instance illustrates the novel ways in which users may adapt their interactions with VAs, transforming routine troubleshooting into a more interactive and enjoyable experience. Similarly, questions such as \textit{``Alexa, are you there?''} or \textit{``Alexa, are you working?''} show a form of human-agent interaction that resembles a ``checking up on'' behavior. 

Our findings expand on existing knowledge by illustrating how smart speaker-based VAs can become integrated and situated within the daily lives of older adults. 
The social interactions with VAs that we captured reveal significant insights; for example, older adults often engage in social niceties with VAs, such as expressing gratitude or greetings (Section \ref{sec:social-responses}), a finding also supported by prior work \cite{pradhan2019phantom}. 
Our findings also align with prior research demonstrating that older adults are more likely to anthropomorphize a virtual agent, often using courteous language to show gratitude, while younger adults generally view virtual agents as more utilitarian tools, focusing primarily on their convenience \cite{oh2020differences, chung2019elderly}.
Expressions of affection toward Alexa---\eg ``I really like you'' or ``I love you''---not only show an emotional attachment that may result in elevated expectations, but also raise ethical concerns about deception, infantilization, and privacy in terms of the nature and impact of such bonds \cite{sharkey2012granny, wachsmuth2018robots}. Given that older adults are a more vulnerable demographic, it is crucial that AI assistance is designed with these potential repercussions in mind.

Furthermore, the use of VAs in situated conversations and as part of social interactions with others (as shown in Section \ref{sec:social-dynamics}) points to their ever-evolving role. Instances when couples involved Alexa in their discussions (C8 and AC5 in Table \ref{tab:alexa-dialogue-private-conversations}) or participants showcased Alexa to visitors (AC3 in Table \ref{tab:alexa-dialogue-private-conversations}) reflect a perception of VAs as active, social entities. 
%Such conversations are also reflective of their impression and mental model of the VA. For instance, C8 shows how the couple P11 has very different mental model from each other since P11a believes that Alexa will be able to answer his question while P11b seems quite sure of the opposite. C9 is an illustrative example of similar mismatch. 
The changing uses and perceptions of VAs among older adults points to their significant role in daily and social activities beyond basic tasks, raising questions about a role that transcends simple assistance; such a shift calls for more discussion around designing VAs to suit the specific needs and preferences of this demographic while considering both ethical aspects and possible improvements. 

%Similarly, Talk2Care, an LLM-powered VA for older adults, improves health information collection and mental support in scenarios such as symptom reporting and post-surgery follow-ups \cite{yang2023talk2care}. Nevertheless, users expressed expectations beyond patient-provider communication, including better integration of the VA with their healthcare management \cite{yang2023talk2care}.

%\subsection{Opportunities, Limitations and Design Considerations for Voice Assistants}
